# Supplementary material for: Concept Matching for Low-Resource Classification
Source: arXiv:2006.00937 source file (2020-06-01)
Supplement: Supplementary file 1 [file 6_appendix.tex]

\appendix
\section{Appendix}

\subsection{Activation function}
\label{appendix:gate}
The activation function of Eq. \ref{eq:gating} controls how similar an embedding and a prototype have to be in order to significantly contribute as a feature. Figure \ref{fig:gating-activation} shows different curves for different values of $a$. A bigger $a$ squashes low cosine similarities more, as is the case for $a=100$, therefore acting as a stricter filter.
\begin{figure}[h]
    \centering
    \includegraphics[width=0.7\textwidth]{images/activations.eps}
    \caption{Plot of the function $g(v) = a^{v-1}$ for different values of $a$. In practice, the argument $v$ will be the cosine similarity between 2 vectors, hence $g: [-1,1] \rightarrow [0,1]$}
    \label{fig:gating-activation}
\end{figure}
For completeness, Figure \ref{fig:gated-2D} shows the effect of a g($\cdot$) in $R^2$, using $a=100$.
\begin{figure}[h]
     \centering
     \begin{subfigure}[b]{0.49\textwidth}
         \centering
         \includegraphics[width=\textwidth]{images/cosine_similarity.eps}
         \caption{Cosine similarity}
         \label{fig:cosine-similarity}
     \end{subfigure}
     \hfill
     \begin{subfigure}[b]{0.49\textwidth}
         \centering
         \includegraphics[width=\textwidth]{images/gated_cosine_similarity.eps}
         \caption{Gated cosine similarity}
         \label{fig:gated-cosine-similarity}
     \end{subfigure}
        \caption{From left to right: (a) Cosine similarity with respect to the [1,1] vector $v$ and (b) its activation for $a=100$. The function acts as a filter on cosine similarity, thus promoting those vectors \quotes{close enough} to $v$ while penalizing the others. }
        \label{fig:gated-2D}
\end{figure}

\newpage
\subsection{Differentiable implementation of AND and OR}
\label{appendix:differentiable-logic}
\begin{figure}[h]
     \centering
     \begin{subfigure}[b]{0.49\textwidth}
         \centering
         \includegraphics[width=\textwidth]{images/AND.eps}
         \caption{Differentiable AND function}
         \label{fig:and}
     \end{subfigure}
     \hfill
     \begin{subfigure}[b]{0.49\textwidth}
         \centering
         \includegraphics[width=\textwidth]{images/OR.eps}
         \caption{Differentiable OR function ($s=2$)}
         \label{fig:or}
     \end{subfigure}
     \hfill
          \begin{subfigure}[b]{0.49\textwidth}
         \centering
         \includegraphics[width=\textwidth]{images/XOR.eps}
         \caption{Differentiable XOR function ($s=2$)}
         \label{fig:xor}
     \end{subfigure}
        \caption{From left to right: Cosine similarity with respect to the [1,1] vector and its gated activation.}
        \label{fig:gated-2D}
\end{figure}
Given the set $\{\phi_1,,\phi_N\} \in [0,1]^N$, interpreted as $N$ \textit{independent} \quotes{soft matching probabilities}, we would like to compute their joint probability as well as the probability of a single matching out of all possible ones. In our experiments, we found a pseudo-differentiable implementation of $min$ and $max$ (Eq. \ref{eq:and-feat} and Eq. \ref{eq:or-feat}) to speed up convergence. Alternatively, we tried a fully differentiable version of those two functions as well as the probability of mutually exclusive events, \ie XOR. We present the equations for $N=2$, although this can be easily generalized to arbitrary $N$:
\begin{align}
& \phi^{Diff}_{AND}(\phi_1, \phi_2) = & \phi_1 * \phi_2 \nonumber \\ \nonumber \\
& \phi^{Diff}_{OR}(\phi_1, \phi_2, s) = & (\phi_1-2)^{-2s} - 2^{-2s}(1-\phi_1) + (\phi_2-2)^{-2s} - 2^{-2s}(1-\phi_2) - \phi^{Diff}_{AND}(\phi_1,\phi_2) \nonumber \\ \nonumber \\
& \phi^{Diff}_{XOR}(\phi_1, \phi_2) = & \phi^{Diff}_{OR}(\phi_1, \phi_2) - \phi^{Diff}_{AND}(\phi_1, \phi_2) \nonumber
\end{align}
where $s$ controls how squashed is the curve is. Figure \ref{fig:gated-2D} depicts all three curves for $s=2$.

\newpage

\subsection{Gradient boosting effect on backpropagation}
For a loss $\ell$ defined on top of Equation \ref{eq:doc-prediction} and a true label $\hat{y}$, backpropagation is computed as (abstracting from the sample index $i$ to simplify notation):

\begin{align}
\frac{\partial \ell(y, \hat{y})}{\partial \boldsymbol{\theta}} = &\frac{\partial \ell(y, \hat{y})}{\partial y} \cdot \frac{\partial y}{\partial \boldsymbol{\theta}} = \frac{\partial \ell(y, \hat{y})}{\partial y} \cdot \frac{\partial \ \sigma(\sum^{T}_j y^jf(r^j))}{\partial (\sum^{T}_j y^jf(r^j))} \cdot \frac{\partial \ \sum^{T}_j y^jf(r^j)}{\partial \boldsymbol{\theta}} \nonumber \\
\frac{\partial \ \sum^{T}_j y^jf(r^j)}{\partial \boldsymbol{\theta}} = &\sum^{T}_j \Big(\frac{\partial (\Delta(x^j)\mathbf{W} + b)}{\partial \boldsymbol{\theta}}\cdot f(r^j)\Big),
\label{eq:error-boosting}
\end{align}
where $\boldsymbol{\theta}$ are the parameters of the model.

\subsection{Robustness to Noise}
\label{appendix:noise-robustness}
\begin{figure}[h]
    \centering
    \includegraphics[width=0.8\textwidth]{images/impact_noise.eps}
    \caption{Robustness to different degrees of rationale noise on the Spouse dataset. From bottom to top, the curves refer to different training sizes: 10, 30, 60, 150, 300. We fix $f(r)=e^r$}
    \label{fig:noise-exp}
\end{figure}
We investigated how injecting random rationales (\ie ones) in prior information affects the final performances. Clearly, having a 100\% noise corresponds to not having rationales at all, therefore we run a simple experiment (with fixed hyper-parameters) 10 times on Spouse, with the goal to study robustness to noise. Figure \ref{fig:noise-exp} shows the result, where different curves stand for different training sizes; as one would expect, for few data points (blue and red curves) noise has bigger influence whereas for 150 (orange curve) and 300 (green curve) data points the effect is negligible. This confirms that there is a trade-off where the impact of rationales has little effect on the final performances.
\newpage
\subsection{Visualization of the most important tokens} 
The importance of tokens in a sentence can be inspected by looking at the prototypes $p_i$, the weight matrix $\mathbf{W}$ and the tokens predictions $y_i^j$. In Figure \ref{fig:implicit-attention} we show the some of the tokens which are responsible for positive prediction on Spouse \textit{unseen} data, which is consistent with the results of Section \ref{explainability}.

\begin{figure}[h]
    \centering
    \includegraphics[width=\textwidth]{images/sentences.png}
    \caption{Visualization of the most important tokens for positive prediction. Sentences were extracted from the Spouse dataset. The entities we are interested in are always called \quotes{alex} and \quotes{chris}.}
    \label{fig:implicit-attention}
\end{figure}
